# Supplementary material for: Large-scale Integration of Experimental and Computational Data for 2D Materials
Source: arXiv:2603.05083 source file (2026-03-05)
Supplement: Supplementary file 1 [file SI.tex]

\documentclass[amsmath,amssymb,prb,twocolumn,superscriptaddress]{revtex4-2}
\usepackage[compatibility=false]{caption}
\usepackage{subcaption}
\usepackage[export]{adjustbox}

\usepackage{pdfpages}

% =======================================

\begin{document}
\clearpage

\section*{}

% Include all pages of your PDF table
\includepdf[pages=-]{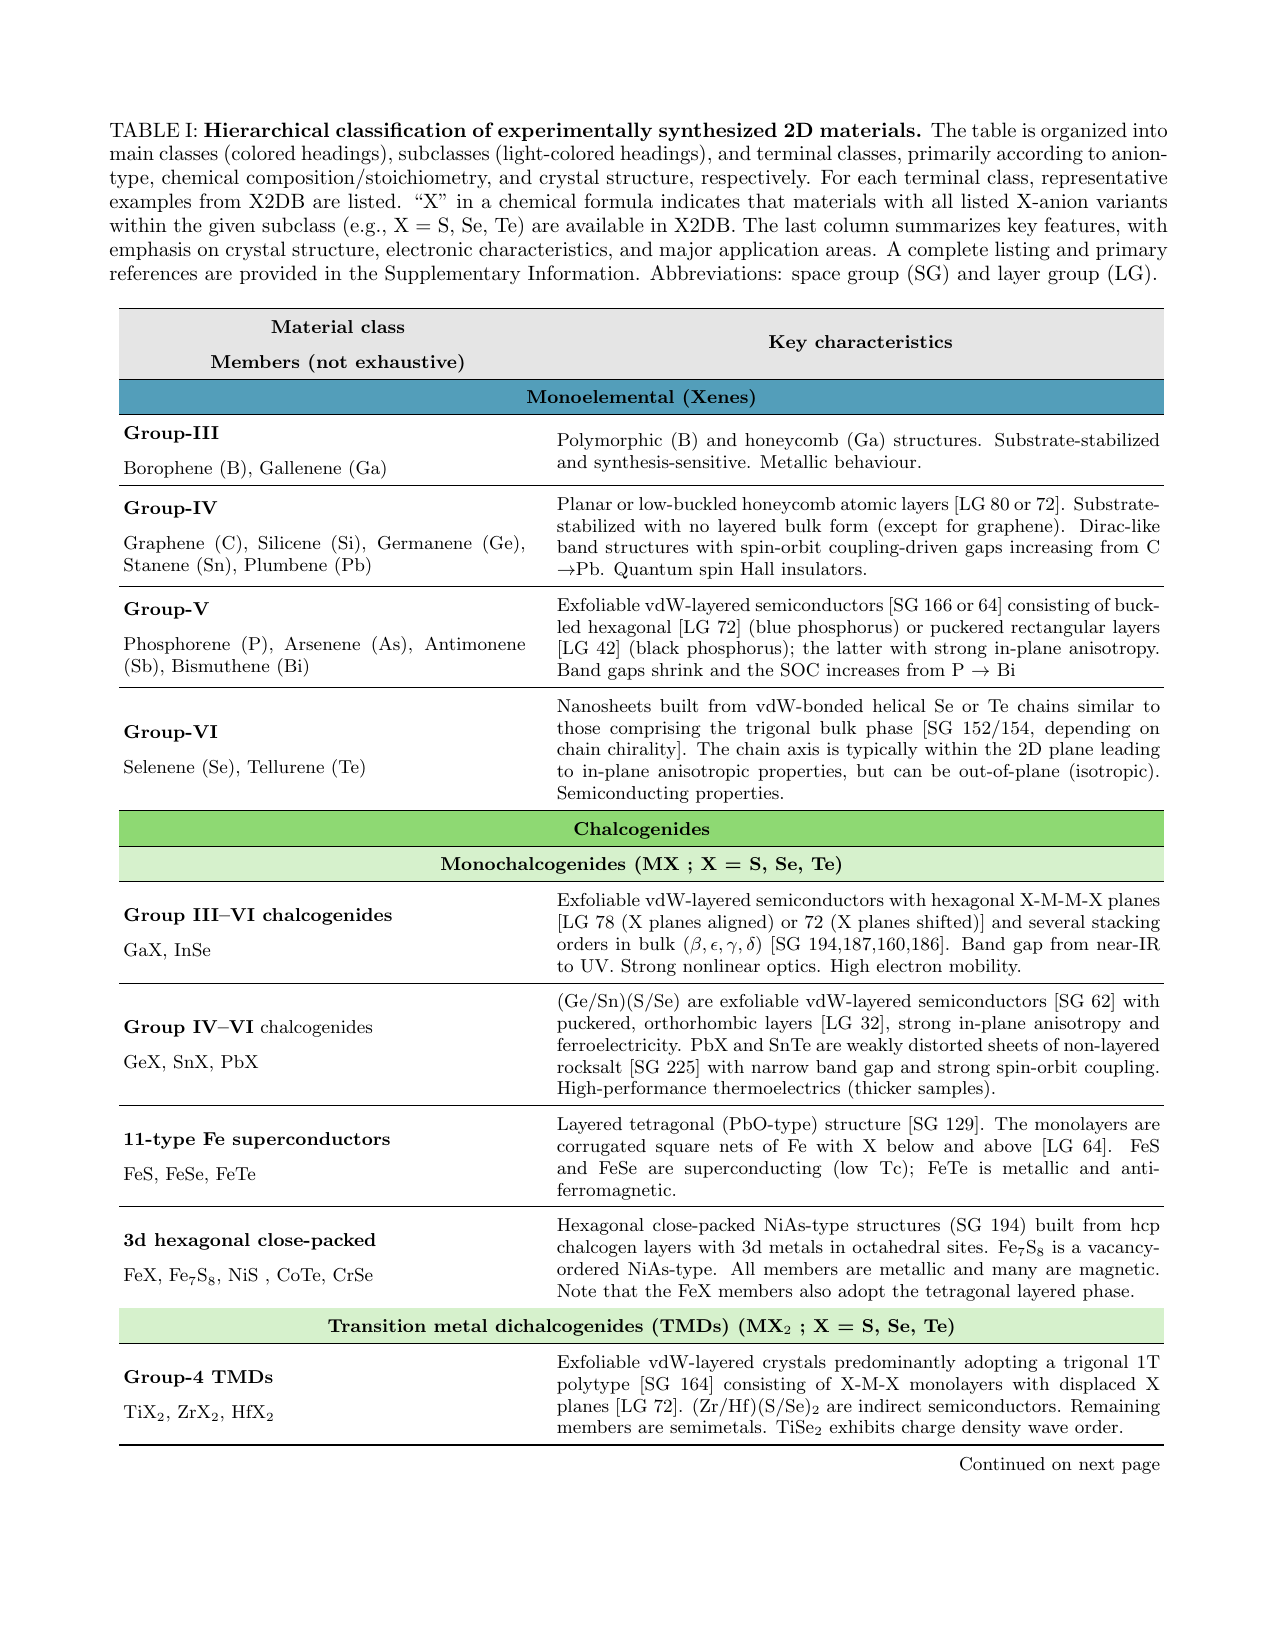}

\end{document}
